# Supplementary material for: CaptainCook4D: A Dataset for Understanding Errors in Procedural Activities
Source: arXiv:2312.14556 source file (2024-12-09)
Supplement: Supplementary file 1 [file early_error_recognition.tex]

\begin{table}[!ht]
\caption{Early Error Category Recognition}
 
\label{tab:early_error_category_recognition}
\resizebox{\columnwidth}{!}{%
\begin{tabular}{cccccc}
\hline
Type of Error                               & \textbf{Method Name} & \textbf{Accuracy} & \textbf{Precision} & \textbf{Recall} & \textbf{F1 Score} \\ \hline
\multirow{5}{*}{\textbf{Technique Error}}   & 3D ResNet            & 90.44             & 27.27              & 4.55            & 7.79              \\
                                            & Slowfast             & 88.83             & 20.69              & 9.09            & 12.63             \\
                                            & X3D                  & 89.77             & 8.33               & 1.52            & 2.56              \\
                                            & VideoMAE             & 89.74             & 30                 & 9.52            & 14.46             \\
                                            & Omnivore             & 87.75             & 20.93              & 13.64           & 16.51             \\ \hline
\multirow{5}{*}{\textbf{Preparation Error}} & 3D ResNet            & 93                & 0                  & 0               & 0                 \\
                                            & Slowfast             & 92.19             & 20.69              & 14.63           & 17.14             \\
                                            & X3D                  & 93.41             & 16.67              & 4.88            & 7.55              \\
                                            & VideoMAE             & 92.34             & 10                 & 5.41            & 7.02              \\
                                            & Omnivore             & 90.85             & 18.6               & 19.51           & 19.05             \\ \hline
\multirow{5}{*}{\textbf{Measurement Error}} & 3D ResNet            & 91.92             & 0                  & 0               & 0                 \\
                                            & Slowfast             & 89.77             & 3.45               & 2.04            & 2.56              \\
                                            & X3D                  & 91.79             & 0                  & 0               & 0                 \\
                                            & VideoMAE             & 90.32             & 0                  & 0               & 0                 \\
                                            & Omnivore             & 88.16             & 4.65               & 4.08            & 4.35              \\ \hline
\multirow{5}{*}{\textbf{Temperature Error}} & 3D ResNet            & 94.58             & 0                  & 0               & 0                 \\
                                            & Slowfast             & 95.4              & 5                  & 25              & 8.33              \\
                                            & X3D                  & 89.94             & 0                  & 0               & 0                 \\
                                            & VideoMAE             & 94                & 3.57               & 20              & 6.06              \\
                                            & Omnivore             & 94.39             & 7.14               & 40              & 12.12             \\ \hline
\multirow{5}{*}{\textbf{Timing Error}}      & 3D ResNet            & 95.29             & 9.09               & 3.85            & 5.41              \\
                                            & Slowfast             & 93.14             & 6.9                & 7.69            & 7.27              \\
                                            & X3D                  & 95.15             & 8.33               & 3.85            & 5.26              \\
                                            & VideoMAE             & 93.64             & 5                  & 3.85            & 4.35              \\
                                            & Omnivore             & 90.98             & 2.33               & 3.85            & 2.9               \\ \hline
\end{tabular}%
}
\end{table}
