# Supplementary material for: CaptainCook4D: A Dataset for Understanding Errors in Procedural Activities
Source: arXiv:2312.14556 source file (2024-12-09)
Supplement: Supplementary file 2 [file error_category_recognition.tex]

\begin{table}[!ht]
\caption{Error Category Recognition}
\label{tab:error_category_recognition}
 
\resizebox{\columnwidth}{!}{%
\begin{tabular}{cccccc}
\hline
Type of Error                               & \textbf{Method Name} & \textbf{Accuracy} & \textbf{Precision} & \textbf{Recall} & \textbf{F1 Score} \\ \hline
\multirow{5}{*}{\textbf{Technique Error}}   & 3D ResNet            & 88.56             & 27.91              & 18.18           & 22.02             \\
                                            & Slowfast             & 82.50             & 19.23              & 30.30           & 23.53             \\
                                            & X3D                  & 83.31             & 9.72               & 10.61           & 10.14             \\
                                            & VideoMAE             & 84.39             & 19.18              & 22.22           & 20.59             \\
                                            & Omnivore             & 78.20             & 17.57              & 39.39           & 24.30             \\ \hline
\multirow{5}{*}{\textbf{Preparation Error}} & 3D ResNet            & 89.77             & 9.30               & 9.76            & 9.52              \\
                                            & Slowfast             & 83.45             & 10.58              & 26.83           & 15.17             \\
                                            & X3D                  & 87.21             & 12.50              & 21.95           & 15.93             \\
                                            & VideoMAE             & 86.99             & 13.70              & 27.03           & 18.18             \\
                                            & Omnivore             & 80.22             & 14.19              & 51.22           & 22.22             \\ \hline
\multirow{5}{*}{\textbf{Measurement Error}} & 3D ResNet            & 88.43             & 6.98               & 6.12            & 6.52              \\
                                            & Slowfast             & 82.10             & 9.62               & 20.41           & 13.07             \\
                                            & X3D                  & 85.33             & 8.33               & 12.24           & 9.92              \\
                                            & VideoMAE             & 84.39             & 8.22               & 12.77           & 10.00             \\
                                            & Omnivore             & 78.33             & 12.16              & 36.73           & 18.27             \\ \hline
\multirow{5}{*}{\textbf{Temperature Error}} & 3D ResNet            & 93.14             & 0.00               & 0.00            & 0.00              \\
                                            & Slowfast             & 85.20             & 0.96               & 12.50           & 1.79              \\
                                            & X3D                  & 89.23             & 0.00               & 0.00            & 0.00              \\
                                            & VideoMAE             & 88.58             & 1.37               & 12.50           & 2.47              \\
                                            & Omnivore             & 79.81             & 2.03               & 37.50           & 3.85              \\ \hline
\multirow{5}{*}{\textbf{Timing Error}}      & 3D ResNet            & 91.52             & 6.98               & 11.54           & 8.70              \\
                                            & Slowfast             & 84.12             & 5.77               & 23.08           & 9.23              \\
                                            & X3D                  & 87.62             & 4.17               & 11.54           & 6.12              \\
                                            & VideoMAE             & 87.14             & 6.85               & 19.23           & 10.10             \\
                                            & Omnivore             & 79.00             & 6.08               & 34.62           & 10.34             \\ \hline
\end{tabular}%
}
\end{table}
